# Supplementary material for: Optimized Non-Primary Channel Access Design in IEEE 802.11bn
Source: arXiv:2405.00227 source file (2024-04-30)
Supplement: Supplementary file 1 [file appendix.tex]

\subsection{Appendix 1}\label{app:1}
